# Supplementary material for: Interlayer binding energy of graphite -- A direct experimental determination
Source: arXiv:1104.1469 source file (2011-04-08)
Supplement: Supplementary file 1 [file Supplementary_information.pdf]

# Supplementary Information

(Dated: April 5, 2011)

This document contains supplementary information to accompany "Interlayer binding energy of graphite – A direct experimental determination" by Liu et al. In these notes, we firstly give a Finite Element Analysis using ABAQUS code and the error estimate of the obtained values, and then we deal with the second sample prepared in scanning electron microscopy (SEM) by atomic force microscopy (AFM) and ABAQUS simulations.

According to Eq. (1), the elastic strain energy of the entire system is required to determine the binding energy. Due to the unique structural and elastic properties of HOPG, i.e., the highest elastic anisotropy and extremely small interlayer shear strength, it is very difficult to analytically determine the strain energy. Instead, we have adopted Finite Element Analysis by using the ABAQUS code.

Consistent to the geometry of the HOPG sample in our experiment, Fig. S1 shows our finite element model, where an elastic plate consist of a $SiO_2$ film of the thickness $h_s$ = 205nm and a graphite flake of thickness $h_g$ = 120nm is spanning over a graphite step of the height $\Delta$ = 30 nm. This elastic $SiO_2$/graphite plate is 'glued' to the bottom surface of the step at given peeling length $L$ in our model. We model our system in a plane strain condition, because the width of the top graphite flake is much larger than the length $L$ and the color of the flake in Fig. 3b suggests deformation quite uniform along the width direction (Fig 3b). In Fig. S1, $y$ axis is perpendicular to the graphite basal plane, $x$ axis and $z$ axis are inside the graphene basal plane and are perpendicular to and parallel to the step contact line, respectively. Young's modulus and Poisson ratio of $SiO_2$ are $E_2$ = 59GPa and $\nu_2$ = 0.24 [1]. The elastic parameters of HOPG [2] are given through the following stress-strain relation:

$$
\begin{Bmatrix} \sigma_x \\ \sigma_y \\ \sigma_z \\ \tau_{yz} \\ \tau_{zx} \\ \tau_{xy} \end{Bmatrix} = \begin{bmatrix} 1060 & 15 & 180 & 0 & 0 & 0 \\ 15 & 36.5 & 15 & 0 & 0 & 0 \\ 180 & 15 & 1060 & 0 & 0 & 0 \\ 0 & 0 & 0 & 2.25 & 0 & 0 \\ 0 & 0 & 0 & 0 & 220 & 0 \\ 0 & 0 & 0 & 0 & 0 & 2.25 \end{bmatrix} \begin{Bmatrix} \varepsilon_x \\ \varepsilon_y \\ \varepsilon_z \\ \gamma_{yz} \\ \gamma_{zx} \\ \gamma_{xy} \end{Bmatrix}, \tag{A1}
$$

where the moduli are given in unit of GPa.

ABAQUS is used to relax our FEM model to obtain the deflection curve $y(x, L)$ of the top surface and the elastic energy $U(L)$. But we find that the shear stress inside such bi-material top flake (shown in Fig. S1) is as large as 10 ~ 90MPa, which is far beyond the interlayer shear strength between graphite layers: ~0.45Mpa [3]. This is because our FEM model used the continuum 2D element to represent the HOPG and thus does not allow the sliding among graphene layers even if the shear stress is beyond the shear strength. Direct simulation of the sliding among graphene layers in ABAQUS is rather challenging. We will show in the following that the HOPG flake can actually be neglected in our ABAQUS model.

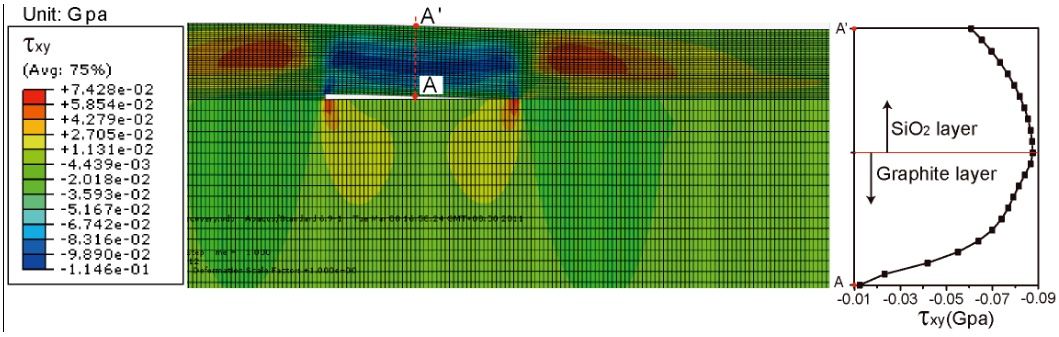


Fig. S1 FEM model of the graphite island sample in experiment, with the shear stress $\tau_{xy}$ distribution calculated by ABAQUS (see text for details).

Due to the extreme contrast between the strong basal plane Young's modulus and ultralow interlayer shear modulus of graphite [4], neither the Euler-Bernoulli's nor the Timoshenko's model was found to be applicable for multilayer graphene beams [5]. We have proved that an $n$-layer graphene beam behaves like an assembly of $n$ monolayer graphene beams with same deflections for all layers [5]. The overall bending rigidity is approximately equal to the $n$ times of the bending rigidity of a monolayer graphene. Thus, we can model the $SiO_2$/graphite plate as an assembly of

bi-beam with the following bending rigidity:

$$D_{\text{bi}} = D_{\text{s}} + nD_{\text{g}} \tag{A2}$$

where $D_s$ and $D_g$ denote the bending rigidities of the $SiO_2$ cover and a monolayer graphene. Using the molecular dynamics simulation result of $D_g \sim 3.4*10^{-19}$ Pa m$^4$ and the layer number estimate $n \approx 360$ (= 120nm/0.335nm), we get $nD_g \approx 0.003*D_s$. We can, therefore, neglect the contribution of the graphene layers below the $SiO_2$ cover to the bending system, i.e., $D_{bi} \approx D_s$.

Figure S2 (a) shows our FEM model without the graphite flake in the spanned top plate. ABAQUS is used to calculate the deflection curve of the top surface and the normal and shear stress distribution. Figure S2(a)-(c) show the results of a sample with $L = 900$nm.

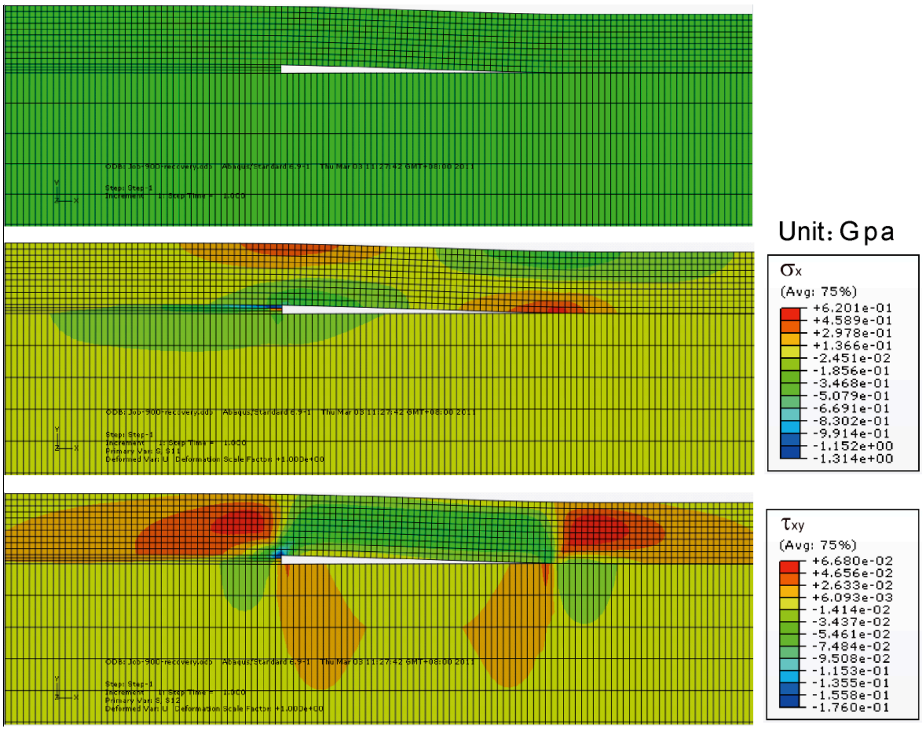


Fig. S2 (a) FEM model of the elastic system depicted in the Insert of Fig. 4, in which the graphite flake is neglected as explained in the text. (b) and (c) show the normal stress $\sigma_x$ and shear stress $\tau_{xy}$ distributions.

We repeat the ABAQUS calculations for our FEM models (Fig. S2(a)) with a set of length $L$. The elastic energies are shown in Fig. 1(b). We then fitted the obtained deflection curves $y(x, L)$ to the AFM measured height profiles shown in Fig. 3(a) and

3(c). Figure S3 depicts the fitting error vs. the length $L$. We determine the peeling length $L$ of the first sample as 890 nm. From Fig. 1(c), we can thus estimate the binding energy as 0.27J/m$^2$.

A possible error bound to the above estimate of bonding energy is analyzed below. The first error comes from the surface roughness of the $SiO_2$ film. The measured thickness of the $SiO_2$ film is 205 ± 8nm. Denote by $h(x) = h_0 + f(x)$, where $h_0$ is the average thickness (205nm) and $f(x)$ is the thickness fluctuation (bounded by 8nm). Therefore, the bending energy of the beam subjected to a pure bending moment $M$ is equal to

$$\begin{aligned} U &= \frac{1}{2}\int_0^L \frac{M^2}{EI}dx = \frac{M^2}{24Eb}\int_0^L \frac{dx}{h^3(x)} \\ &= \frac{6M^2}{Eb}\int_0^L \frac{dx}{h_0^3(1+f/h_0)^3} \\ &= \frac{6M^2}{Ebh_0^3}\int_0^L (1-3\frac{f}{h_0}+6\frac{f^2}{h_0^2}+...)dx \\ &\approx \frac{6M^2L}{Ebh_0^3}(1+6\frac{\overline{f}^2}{h_0^2}) \end{aligned} \tag{A3}$$

where $\overline{f}^2$ denotes the average value of $f^2(x)$. It differs from the strain energy $U_0$ stored in the beam with the constant thickness $h_0$ a relative error $6\overline{f}^2/h_0^2$, which is about 6*(8nm/205nm) ≈ 0.9%. Therefore, we can ignore the influence of the measured surface roughness.

Secondly, we give an estimate of the possible error resulted by a span length uncertainty. The total strain energy stored in the spanned beam is known to be

$$U = \frac{6EI\Delta^2}{L^3} \tag{A4}$$

Therefore, the relative error resulted by spanned length uncertainty $\delta L$ can be estimated as

$$\frac{\delta U}{U} = -3\frac{\delta L}{L} \tag{A5}$$

In our AFM measurement, the resolution in the scanning plane is about 20nm. Therefore, the possible upper relative error bound is 3*(20nm/890nm) ≈ 6.7%.

Thus the overall relative error bound would be about 8%, yielding the bonding

energy of $0.27 \pm 0.02$ J/m$^2$.

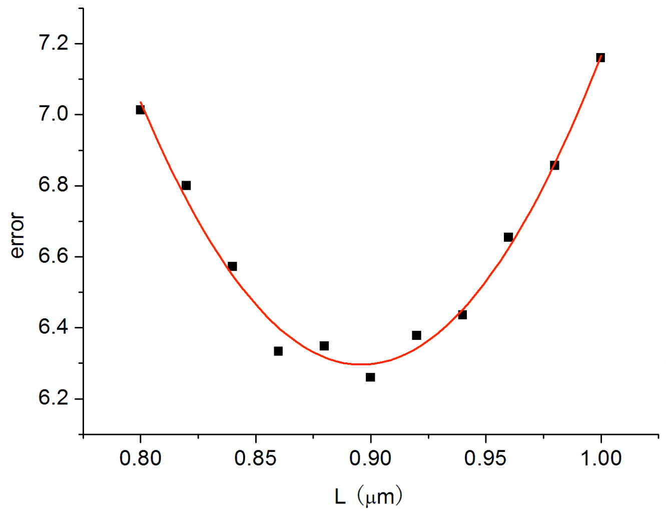


Fig. S3 The black dots corresponding to the errors obtained by least square fitting the deflection curves *y(x, L)* from FEM to the AFM measured height profiles in Fig. 4(a), while the red line is the fitted result of this datum.

Figure S4(a) shows the AFM image of the second sample prepared in SEM under a high vacuum condition. The thickness of the $SiO_2$ thin film is 138±4 nm. Figure S4(b) shows the height profile along the black line in Fig. S4(a). Following the similar FEM analysis as the first sample and using the geometry parameters determined from our AFM measurement, we calculate the deflection curves and the elastic energy of the whole system at a set of length *L*. Figure S4(c) presents the elastic energy vs. peeling length L and Fig. S4(d) shows the calculated binding energy vs. length *L*. Fitting the AFM measured height profile to the ABAQUS determined deflection curves *y(x, L)* leads to the *L*=682nm with the minimal fitting error (Fig. S5), which is taken as the peeling length of this sample. We can then determine the binding energy as 0.30J/m$^2$ from Fig. S4(d). If we take the resolution of our AFM scan (i.e., 20nm) as the uncertainty on *L*, we can estimate the error bound on binding energy as 0.025J/m$^2$. It is worth noting that in the second sample, we find some additional peelings occur in the top surface of the middle flake (Fig. S4(a)). So the surface could not be

completely flat, which results in subtle height difference at different positions as we observed in our AFM scan. Our FEM model cannot very accurately describe this second sample and the determined binding energy is thus less reliable than the value determined in our first sample.

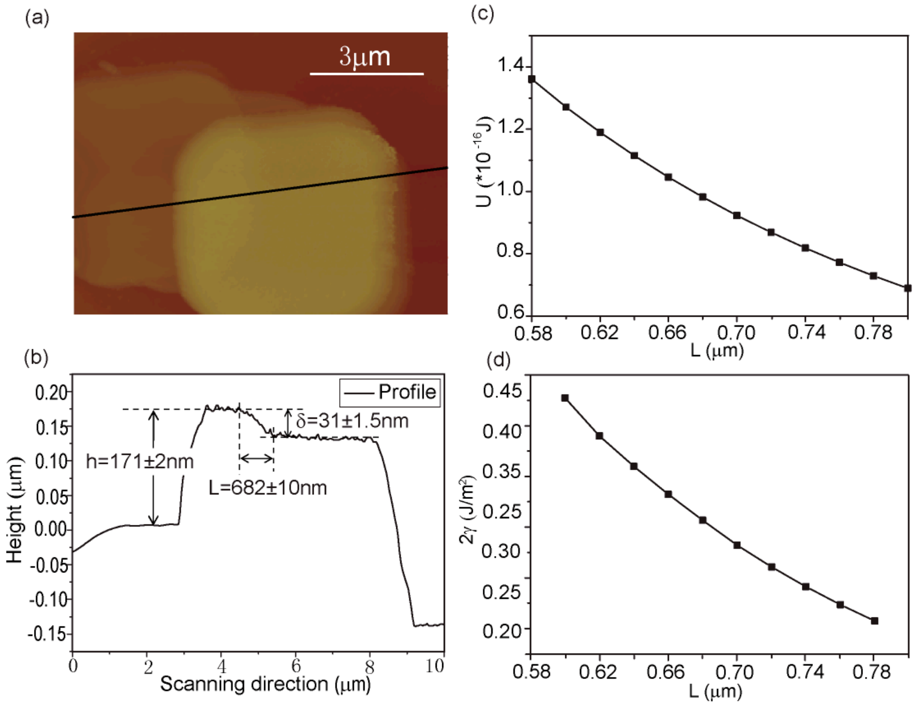


Fig.S4 (a) AFM image of the second sample prepared in SEM. (b) Geometry profile along the black line in (a) with the parameters labeled, where the error bar is calculated from a few of such profiles. (c) Elastic strain energy of the whole system calculated by ABAQUS model with geometry parameters labeled in (b). (d). The binding energy obtained by central finite difference of the datum in (c).

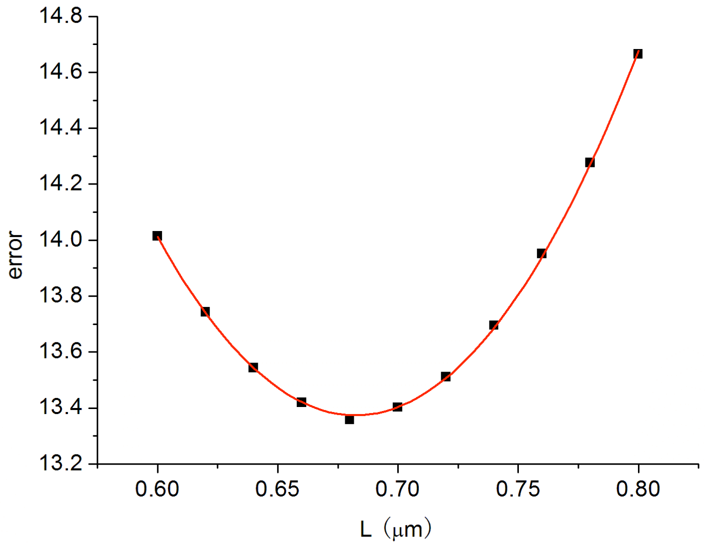


Fig.S5 (a) AFM image of the second sample prepared in SEM. The black dots corresponding to the errors obtained by least square fitting the deflection curves $y(x, L)$ from FEM to the AFM measured height profiles in Fig. S4(a), while the red line is the fitted result of this datum.

[1] J. H. Zhao, et.al., J. Appl. Phys., 85, 6421(1999).

[2] B. T. Kelly, Physics of Graphite (Applied Science, London,1981).

[3] D. E. Soule, C. W. Nezbeda, J. Appl. Phys. 39, 5122 (1968).

[4] L. F. Wang, et.al., Appl. Phys. Lett. 90, 153113 (2007).

[5] Yilun Liu., et. al., Effect of interlayer shear to graphene resonators, J. Mech. Phys. Solids (revised version under review, see also: http://arxiv.org/abs/1012.0766).
